# Supplementary material for: Putting Recommendations on the Map -- Visualizing Clusters and Relations
Source: arXiv:0906.5286 source file (2009-06-29)
Supplement: Supplementary file 1 [file appendix.tex]

\begin{appendix}
The appendix contains zoomed-in areas of the countries described in Sections \ref{sec_tvland} and \ref{sec_lastfm}.  All the images are available at \url{www.research.att.com/~volinsky/maps}.

%\begin{figure}[!htb]
%\begin{center}
%\includegraphics*[width=8cm, angle = 0]{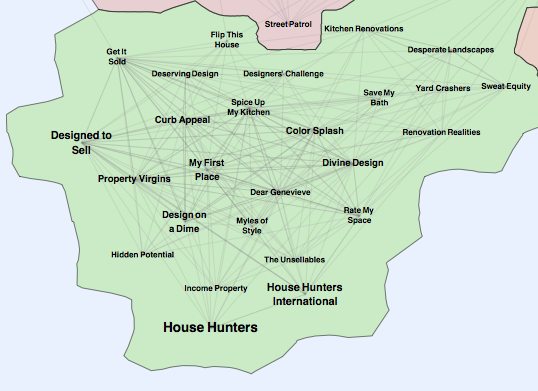}
%\caption{\small\sf Renovation Nation\label{renovation}}
%\end{center}
%\end{figure}

%\begin{figure}[!htb]
%\begin{center}
%\includegraphics*[width=8cm, angle = 0]{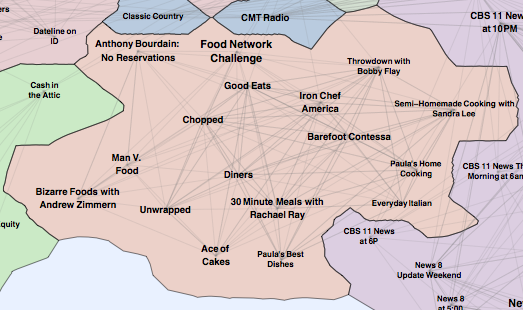}
%\caption{\small\sf Hung'ry\label{hungry}}
%\end{center}
%\end{figure}

\begin{figure}[!htb]
\begin{center}
\includegraphics*[width=8cm, angle = 0]{DATA/uverse_1000_middlelands}
\vspace{-.3cm}
\caption{\small\sf TV Middlelands\label{middlelands}}
\end{center}
\end{figure}

\begin{figure}[!htb]
\begin{center}
\vspace{-.3cm}
\includegraphics*[width=8cm, angle = 0]{DATA/uverse_1000_lowlands}
\vspace{-.3cm}
\caption{\small\sf TV Lowlands\label{lowlands}}
\end{center}
\end{figure}

\begin{figure}[!htb]
\begin{center}
\vspace{-.3cm}
\includegraphics*[width=8cm, angle = 0]{DATA/last_fm_2000_female}
\vspace{-.3cm}
\caption{\small\sf Female singer-songwriter cluster\label{female}}
\end{center}
\end{figure}

\begin{figure}[!htb]
\begin{center}
\vspace{-.3cm}
\includegraphics*[width=5cm, angle = 0]{DATA/last_fm_2000_beatles}
\vspace{-.3cm}
\caption{\small\sf Beatles cluster\label{beatles}}
\end{center}
\end{figure}

\begin{figure}[!htb]
\begin{center}
\includegraphics*[width=8cm, angle = 0]{DATA/last_fm_2000_metallands}
\vspace{-.3cm}
\caption{\small\sf Music Metallands\label{metallands}}
\end{center}
\end{figure}

\begin{figure}[!htb]
\begin{center}
\includegraphics*[width=8.5cm, angle = 0]{DATA/last_fm_2000_grungeland}
\vspace{-.3cm}
\caption{\small\sf Music Grungelands\label{grungelands}}
\end{center}
\end{figure}

\begin{figure}[!htb]
\begin{center}
\includegraphics*[width=8cm, angle = 0]{DATA/last_fm_2000_indyana}
\vspace{-.3cm}
\caption{\small\sf Indyana\label{indyana}}
\end{center}
\end{figure}

\begin{figure*}
\begin{center}
\includegraphics[width=16cm, angle = 0]{DATA/uverse_1000_toddlersprawl}
\vspace{-.3cm}
\caption{\small\sf TV ToddlerSprawl\label{toddlersprawl}}
\end{center}
\end{figure*}

\begin{figure*}
\begin{center}
\includegraphics[width=16cm, angle = 0]{DATA/uverse_1000_premium}
\vspace{-.3cm}
\caption{\small\sf TV Premium Peninsula\label{premium}}
\end{center}
\end{figure*}

\end{appendix}
